# Supplementary material for: Neuro-mimetic Task-free Unsupervised Online Learning with Continual Self-Organizing Maps
Source: arXiv:2402.12465 source file (2024-02-19)
Supplement: Supplementary file 1 [file Cont-SOM_model.pdf]

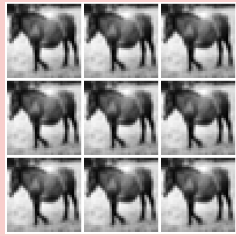

tilled input  
without label

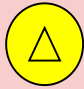

element-wise  
distance

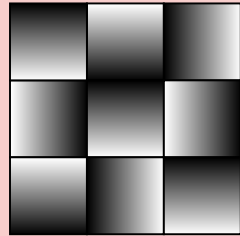

randomly initialized  
untrained ContSOM

min  
pool

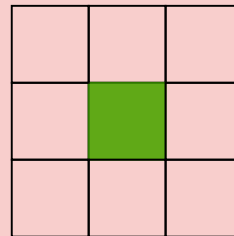

Best Matching Unit (BMU)

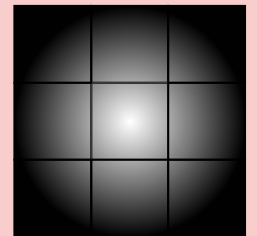

Update Mask in the  
neighborhood of BMU

Weig  
upda

Repeat for next input sample

ht  
te

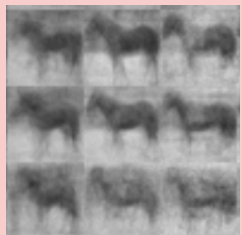

trained contSOM
